# Supplementary material for: Stochastic Training of Graph Convolutional Networks with Variance Reduction
Source: arXiv:1710.10568 source file (2018-03-01)
Supplement: Supplementary file 1 [file supplementary.pdf]

# Stochastic Training of Graph Convolutional Networks with Variance Reduction: Supplementary Material

## A Derivation of the variance

The following proposition is widely used in this section.

**Proposition A.** *Let $X_1, \dots, X_N$ are random variables, then*

$$Var\left[\sum_{i=1}^{N} X_i\right] = \sum_{i=1}^{N}\sum_{j=1}^{N} Cov\left[X_i, X_j\right].$$

*Proof.*

$$\begin{aligned}
\text{Var}\left[\sum_{i=1}^{N} X_i\right] &= \mathbb{E}\left[\sum_{i=1}^{N}\sum_{j=1}^{N} X_i X_j\right] - \left(\mathbb{E}\sum_{i=1}^{N} X_i\right)^2 \\
&= \mathbb{E}\left[\sum_{i=1}^{N}\sum_{j=1}^{N} \left(X_i X_j - \frac{1}{N}\mathbb{E}\sum_{i=1}^{N} X_i\right)\right] \\
&= \sum_{i=1}^{N}\sum_{j=1}^{N} \text{Cov}\left[X_i, X_j\right].
\end{aligned}$$

□

We begin with the proof for the three propositions in the main text.

**Proposition 1.** *If $\hat{\mathbf{n}}^{(l)}(u)$ contains $D^{(l)}$ samples from $\mathbf{n}(u)$ without replacement, then $Var_{\hat{\mathbf{n}}^{(l)}(u)}\left[\frac{n(u)}{D^{(l)}}\sum_{v\in\hat{\mathbf{n}}^{(l)}(u)} x_v\right] = \frac{C_u^{(l)}}{2D^{(l)}}\sum_{v_1\in\mathbf{n}(u)}\sum_{v_2\in\mathbf{n}(u)}(x_{v_1}-x_{v_2})^2$, where $C_u^{(l)} = 1-(D^{(l)}-1)/(n(u)-1)$.*

*Proof.* We denote the $D^{(l)}$ samples in the set as $v_1, \dots, v_{D^{(l)}}$.Let $\bar{x} = \frac{1}{n(u)}\sum_{v\in\mathbf{n}(u)} x_v$,

then

$$
\begin{aligned}
&\mathrm{Var}_{\hat{\mathbf{n}}^{(l)}(u)}\left[\frac{n(u)}{D^{(l)}}\sum_{v\in\hat{\mathbf{n}}^{(l)}(u)}x_v\right]\\
=&\mathrm{Var}_{v_1,\ldots,v_{D^{(l)}}}\left[\frac{n(u)}{D^{(l)}}\sum_{i=1}^{D^{(l)}}x_{v_i}\right]\\
=&\left(\frac{n(u)}{D^{(l)}}\right)^2\sum_{i=1}^{D^{(l)}}\sum_{j=1}^{D^{(l)}}\mathrm{Cov}_{v_1,\ldots,v_{D^{(l)}}}\left[x_{v_i},x_{v_j}\right]\\
=&\left(\frac{n(u)}{D^{(l)}}\right)^2\left\{\sum_{i=1}^{D^{(l)}}\mathrm{Var}_{v_i}\left[x_{v_i}^2\right]+\sum_{i\neq j}\mathrm{Cov}_{v_i,v_j}\left[x_{v_i},x_{v_j}\right]\right\}\\
=&\left(\frac{n(u)}{D^{(l)}}\right)^2\left\{\frac{D^{(l)}}{n(u)}\sum_{v\in\mathbf{n}(u)}(x_v-\bar{x})^2+\frac{D^{(l)}(D^{(l)}-1)}{n(u)(n(u)-1)}\left[\sum_{i,j\in\mathbf{n}(u)}(x_i-\bar{x})(x_j-\bar{x})-\sum_{i\in\mathbf{n}(u)}(x_i-\bar{x})^2\right]\right\}\\
=&\frac{n(u)}{D^{(l)}}\left(1-\frac{D^{(l)}-1}{n(u)-1}\right)\left(\sum_{v\in\mathbf{n}(u)}x_v^2-n(u)\bar{x}^2\right)\\
=&\frac{1}{2D^{(l)}}\left(1-\frac{D^{(l)}-1}{n(u)-1}\right)\left(2n(u)\sum_{v\in\mathbf{n}(u)}x_v^2-\sum_{v_1,v_2\in\mathbf{n}(u)}2x_{v_1}x_{v_2}\right)\\
=&\frac{C_u^{(l)}}{2D^{(l)}}\sum_{v_1,v_2\in\mathbf{n}(u)}(x_{v_1}-x_{v_2})^2.
\end{aligned}
$$

□

**Proposition 2.** *If $\hat{\mathbf{n}}^{(l)}(u)$ contains $D^{(l)}$ samples from the set $\mathbf{n}(u)$ without replacement, $x_1,\ldots,x_V$ are random variables, $\forall v, \mathbb{E}\left[x_v\right]=0$ and $\forall v_1\neq v_2$, $Cov\left[x_{v_1},x_{v_2}\right]=0$, then $Var_{X,\hat{\mathbf{n}}^{(l)}(u)}\left[\frac{n(u)}{D^{(l)}}\sum_{v\in\hat{\mathbf{n}}^{(l)}(u)}x_v\right]=\frac{n(u)}{D^{(l)}}\sum_{v\in\mathbf{n}(u)}Var\left[x_v\right].$*

*Proof.*

$$
\begin{aligned}
&\mathrm{Var}_{X,\hat{\mathbf{n}}^{(l)}(u)}\left[\frac{n(u)}{D^{(l)}}\sum_{v\in\hat{\mathbf{n}}^{(l)}(u)} x_v\right] \\
=&\left(\frac{n(u)}{D^{(l)}}\right)^2 \mathbb{E}_X\left\{\sum_{i=1}^{D^{(l)}}\mathbb{E}_{\hat{\mathbf{n}}^{(l)}(u)}x_{v_i}^2+\sum_{i\neq j}\mathbb{E}_{\hat{\mathbf{n}}^{(l)}(u)}x_{v_i}x_{v_j}\right\} \\
=&\left(\frac{n(u)}{D^{(l)}}\right)^2 \mathbb{E}_X\left\{\frac{D^{(l)}}{n(u)}\sum_{i\in\mathbf{n}(u)}x_i^2+\frac{D^{(l)}(D^{(l)}-1)}{n(u)(n(u)-1)}\sum_{i,j\in\mathbf{n}(u),i\neq j}x_ix_j\right\} \\
=&\frac{n(u)}{D^{(l)}}\sum_{i\in\mathbf{n}(u)}\mathrm{Var}\left[x_i\right].
\end{aligned}
$$

□

**Proposition 3.** *$X$ and $Y$ are two random variables, and $f(X,Y)$ and $g(Y)$ are two functions. If $E_X f(X,Y)=0$, then $Var_{X,Y}\left[f(X,Y)+g(Y)\right]=Var_{X,Y}f(X,Y)+$ $Var_Y g(Y)$.*

*Proof.*

$$
\mathrm{Var}_{X,Y}\left[f(X,Y)+g(Y)\right]=\mathrm{Var}_{X,Y}f(X,Y)+\mathrm{Var}_Y g(Y)+2\mathrm{Cov}_{X,Y}[f(X,Y),g(Y)],
$$

where

$$
\begin{aligned}
\mathrm{Cov}_{X,Y}[f(X,Y),g(Y)] &= \mathbb{E}_Y\mathbb{E}_X\left[(f(X,Y)-\mathbb{E}_{X,Y}f(X,Y))(g(Y)-E_Y g(Y))\right] \\
&= \mathbb{E}_Y\left[(\mathbb{E}_X f(X,Y)-0)(g(Y)-E_Y g(Y))\right] \\
&= \mathbb{E}_Y\left[0(g(Y)-E_Y g(Y))\right]=0.
\end{aligned}
$$

□

Then, we derive the variance of the estimators with dropout is present.

## A.1 Variance of the exact estimator

$$
\mathrm{Var}_M\left[\sum_{v\in\mathbf{n}(u)}P_{uv}h_v^{(l)}\right]=\mathrm{Var}_M\left[\sum_{v\in\mathbf{n}(u)}P_{uv}\mathring{h}_v^{(l)}\right]=\sum_{v\in\mathbf{n}(u)}P_{uv}^2\mathrm{Var}_M\left[\mathring{h}_v^{(l)}\right]=S_u^{(l)}.
$$

## A.2 Variance of the NS estimator

$$
\begin{aligned}
&\operatorname{Var}_{\hat{\mathbf{n}}^{(l)}(u),M}\left[\mathrm{NS}_u^{(l)}\right]\\
=&\operatorname{Var}_{\hat{\mathbf{n}}^{(l)}(u),M}\left[\frac{n(u)}{D^{(l)}}\sum_{v\in\hat{\mathbf{n}}^{(l)}(u)} P_{uv}h_v^{(l)}\right]\\
=&\operatorname{Var}_{\hat{\mathbf{n}}^{(l)}(u),M}\left[\frac{n(u)}{D^{(l)}}\sum_{v\in\hat{\mathbf{n}}^{(l)}(u)} P_{uv}(\mathring{h}_v^{(l)}+\mu_v^{(l)})\right]\\
=&\operatorname{Var}_{\hat{\mathbf{n}}^{(l)}(u),M}\left[\frac{n(u)}{D^{(l)}}\sum_{v\in\hat{\mathbf{n}}^{(l)}(u)} P_{uv}\mathring{h}_v^{(l)}\right]+\operatorname{Var}_{\hat{\mathbf{n}}^{(l)}(u)}\left[\frac{n(u)}{D^{(l)}}\sum_{v\in\hat{\mathbf{n}}^{(l)}(u)} P_{uv}\mu_v^{(l)}\right],
\end{aligned}
$$

where the last equality is by Proposition 3. By Proposition 2, VD is

$$
\begin{aligned}
&\operatorname{Var}_{\hat{\mathbf{n}}^{(l)}(u),M}\left[\frac{n(u)}{D^{(l)}}\sum_{v\in\hat{\mathbf{n}}^{(l)}(u)} P_{uv}\mathring{h}_v^{(l)}\right]\\
=&\operatorname{Var}_M\operatorname{Var}_{\hat{\mathbf{n}}^{(l)}(u)}\left[\frac{n(u)}{D^{(l)}}\sum_{v\in\hat{\mathbf{n}}^{(l)}(u)} P_{uv}\mathring{h}_v^{(l)}\right]\\
=&\frac{n(u)}{D^{(l)}}S_u^{(l)},
\end{aligned}
$$

where $S_u^{(l)}=\sum_{v\in\mathbf{n}(u)}\operatorname{Var}_M\left[P_{uv}h_v^{(l)}\right]$ is defined in Sec. 5.2. By Proposition 1, VNS is

$$
\operatorname{Var}_{\hat{\mathbf{n}}^{(l)}(u)}\left[\frac{n(u)}{D^{(l)}}\sum_{v\in\hat{\mathbf{n}}^{(l)}(u)} P_{uv}\mu_v^{(l)}\right]=\frac{C_u^{(l)}}{2D^{(l)}}\sum_{v_1,v_2\in\mathbf{n}(u)}(P_{uv_1}\mu_{v_1}^{(l)}-P_{uv_2}\mu_{v_2}^{(l)})^2.
$$

## A.3 Variance of the CVD estimator

$$
\begin{aligned}
&\operatorname{Var}_{\hat{\mathbf{n}}^{(l)}(u),M}\left[\mathrm{CVD}_u^{(l)}\right]\\
=&\operatorname{Var}_{\hat{\mathbf{n}}^{(l)}(u),M}\left[\sqrt{\frac{n(u)}{D^{(l)}}}\sum_{v\in\hat{\mathbf{n}}^{(l)}(u)} P_{uv}\mathring{h}_v^{(l)}+\frac{n(u)}{D^{(l)}}\sum_{v\in\hat{\mathbf{n}}^{(l)}(u)} P_{uv}\Delta\mu_v^{(l)}+\sum_{v\in\mathbf{n}(u)}P_{uv}\bar{\mu}_v^{(l)}\right]\\
=&\operatorname{Var}_{\hat{\mathbf{n}}^{(l)}(u),M}\left[\sqrt{\frac{n(u)}{D^{(l)}}}\sum_{v\in\hat{\mathbf{n}}^{(l)}(u)} P_{uv}\mathring{h}_v^{(l)}\right]+\operatorname{Var}_{\hat{\mathbf{n}}^{(l)}(u)}\left[\frac{n(u)}{D^{(l)}}\sum_{v\in\hat{\mathbf{n}}^{(l)}(u)} P_{uv}\Delta\mu_v^{(l)}+\sum_{v\in\mathbf{n}(u)}P_{uv}\bar{\mu}_v^{(l)}\right],
\end{aligned}
$$

where the last equality is by Proposition 3. By Proposition 2, VD is

$$
\begin{aligned}
&\mathrm{Var}_{\hat{\mathbf{n}}^{(l)}(u),M}\left[\sqrt{\frac{n(u)}{D^{(l)}}}\sum_{v\in\hat{\mathbf{n}}^{(l)}(u)}P_{uv}\mathring{h}_v^{(l)}\right]\\
=&\frac{D^{(l)}}{n(u)}\mathrm{Var}_M\mathrm{Var}_{\hat{\mathbf{n}}^{(l)}(u)}\left[\frac{n(u)}{D^{(l)}}\sum_{v\in\hat{\mathbf{n}}^{(l)}(u)}P_{uv}\mathring{h}_v^{(l)}\right]\\
=&S_u^{(l)}.
\end{aligned}
$$

By Proposition 1, VNS is

$$
\begin{aligned}
&\mathrm{Var}_{\hat{\mathbf{n}}^{(l)}(u)}\left[\frac{n(u)}{D^{(l)}}\sum_{v\in\hat{\mathbf{n}}^{(l)}(u)}P_{uv}\Delta\mu_v^{(l)}+\sum_{v\in\mathbf{n}(u)}P_{uv}\bar{\mu}_v^{(l)}\right]\\
=&\mathrm{Var}_{\hat{\mathbf{n}}^{(l)}(u)}\left[\frac{n(u)}{D^{(l)}}\sum_{v\in\hat{\mathbf{n}}^{(l)}(u)}P_{uv}\Delta\mu_v^{(l)}\right]\\
=&\frac{C_u^{(l)}}{2D^{(l)}}\sum_{v_1,v_2\in\mathbf{n}(u)}(P_{uv_1}\Delta\mu_{v_1}^{(l)}-P_{uv_2}\Delta\mu_{v_2}^{(l)})^2.
\end{aligned}
$$

## A.4 Variance of the CV estimator

$$
\begin{aligned}
&\mathrm{Var}_{\hat{\mathbf{n}}^{(l)}(u),M}\left[\mathrm{CV}_u^{(l)}\right]\\
=&\mathrm{Var}_{\hat{\mathbf{n}}^{(l)}(u),M}\left[\frac{n(u)}{D^{(l)}}\sum_{v\in\hat{\mathbf{n}}^{(l)}(u)}P_{uv}\Delta h_v^{(l)}+\sum_{v\in\mathbf{n}(u)}P_{uv}\bar{h}_v^{(l)}\right]\\
=&\mathrm{Var}_{\hat{\mathbf{n}}^{(l)}(u),M}\left[\frac{n(u)}{D^{(l)}}\sum_{v\in\hat{\mathbf{n}}^{(l)}(u)}P_{uv}\Delta\mathring{h}_v^{(l)}+\sum_{v\in\mathbf{n}(u)}P_{uv}\bar{\mathring{h}}_v^{(l)}+\frac{n(u)}{D^{(l)}}\sum_{v\in\hat{\mathbf{n}}^{(l)}(u)}P_{uv}\Delta\mu_v^{(l)}+\sum_{v\in\mathbf{n}(u)}P_{uv}\bar{\mu}_v^{(l)}\right]\\
=&\mathrm{Var}_{\hat{\mathbf{n}}^{(l)}(u),M}\left[\frac{n(u)}{D^{(l)}}\sum_{v\in\hat{\mathbf{n}}^{(l)}(u)}P_{uv}\Delta\mathring{h}_v^{(l)}+\sum_{v\in\mathbf{n}(u)}P_{uv}\bar{\mathring{h}}_v^{(l)}\right]\\
&+\mathrm{Var}_{\hat{\mathbf{n}}^{(l)}(u)}\left[\frac{n(u)}{D^{(l)}}\sum_{v\in\hat{\mathbf{n}}^{(l)}(u)}P_{uv}\Delta\mu_v^{(l)}+\sum_{v\in\mathbf{n}(u)}P_{uv}\bar{\mu}_v^{(l)}\right],
\end{aligned}
$$

where $\Delta\mathring{h}_v^{(l)}=(h_v^{(l)}-\mu_v^{(l)})-(\bar{h}_v^{(l)}-\bar{\mu}_v^{(l)})$, and the last equality is by Proposition 3. The VNS term is the same with CVD's VNS term.

To analyze the VD, we further assume $\bar{\mathring{h}}_v^{(l)}$ and $\mathring{h}_v^{(l)}$ are i.i.d., so $\mathbb{E}_M\Delta\mathring{h}_v^{(l)}=0$,

$\mathbb{E}_M(\Delta \mathring{h}_v^{(l)})^2 = 2\mathbb{E}_M(\mathring{h}_v^{(l)})^2$, and $\mathbb{E}_M \mathring{h}_v^{(l)} \Delta \mathring{h}_v^{(l)} = \mathbb{E}_M(\mathring{h}_v^{(l)})^2$.

$$
\begin{aligned}
&\mathrm{Var}_{\hat{\mathbf{n}}^{(l)}(u),M}\left[\frac{n(u)}{D^{(l)}}\sum_{v\in\hat{\mathbf{n}}^{(l)}(u)} P_{uv}\Delta\mathring{h}_v^{(l)} + \sum_{v\in\mathbf{n}(u)} P_{uv}\bar{\mathring{h}}_v^{(l)}\right] \\
=&\mathbb{E}_{\hat{\mathbf{n}}^{(l)}(u),M}\Big\{\left(\frac{n(u)}{D^{(l)}}\right)^2 \sum_{i,j\in\hat{\mathbf{n}}^{(l)}(u)} P_{ui}P_{uj}\Delta\mathring{h}_i^{(l)}\Delta\mathring{h}_j^{(l)} + \sum_{i,j\in\mathbf{n}(u)} P_{ui}P_{uj}\bar{\mathring{h}}_i^{(l)}\bar{\mathring{h}}_j^{(l)} \\
&+ 2\frac{n(u)}{D^{(l)}} \sum_{i\in\hat{\mathbf{n}}^{(l)}(u), j\in\mathbf{n}(u)} P_{ui}P_{uj}\Delta\mathring{h}_i^{(l)}\bar{\mathring{h}}_j^{(l)}\Big\} \\
=&\left(\frac{n(u)}{D^{(l)}}\right)^2 \sum_{i\in\hat{\mathbf{n}}^{(l)}(u)} \mathbb{E}_{\hat{\mathbf{n}}^{(l)}(u),M}(P_{ui}\Delta\mathring{h}_i^{(l)})^2 + \sum_{i\in\mathbf{n}(u)} P_{ui}^2\mathbb{E}_M\bar{\mathring{h}}_i^{(l)} + 2\sum_{ij\in\mathbf{n}(u)} P_{ui}P_{uj}\Delta\mathring{h}_i^{(l)}\bar{\mathring{h}}_j^{(l)} \\
=&\frac{n(u)}{D^{(l)}}\sum_{i\in\mathbf{n}(u)} P_{ui^2}\mathbb{E}_M(\mathring{h}_i^{(l)})^2 + \sum_{i\in\mathbf{n}(u)} P_{ui}^2\mathbb{E}_M\bar{\mathring{h}}_i^{(l)} + 2\sum_{i\in\mathbf{n}(u)} P_{ui}^2\mathbb{E}_M\bar{\mathring{h}}_i^{(l)} \\
=&\left(3+\frac{n(u)}{D^{(l)}}\right)S_u^{(l)}.
\end{aligned}
$$

# B Proof of Theorem 1

**Theorem 1.** *For a constant sequence of $W_i = W$ and any $i > LI$ (i.e., after $L$ epochs), the activations computed by CV are exact, i.e., $Z_{CV,i}^{(l)} = Z^{(l)}$ for each $l \in [L]$ and $H_{CV,i}^{(l)} = H^{(l)}$ for each $l \in [L-1]$.*

*Proof.* We prove by induction. After the first epoch the activation $h_{i,v}^{(0)}$ is at least computed once for each node $v$. So $\bar{H}_{CV,i}^{(0)} = H_{CV,i}^{(0)} = H^{(0)} = X$ for all $i > I$. Assume that we have $\bar{H}_{CV,i}^{(l)} = H_{CV,i}^{(l)} = H^{(l)}$ for all $i > (l+1)I$. Then for all $i > (l+1)I$

$$
Z_{CV,i}^{(l+1)} = \left(\hat{P}_i^{(l)}(H_{CV,i}^{(l)} - \bar{H}_{CV,i}^{(l)}) + P\bar{H}_{CV,i}^{(l)}\right)W^{(l)} = P\bar{H}_{CV,i}^{(l)}W^{(l)} = PH^{(l)}W^{(l)} = Z^{(l+1)}. \quad (1)
$$

$$
H_{CV,i}^{(l+1)} = \sigma(Z_{CV,i}^{(l+1)}) = H^{(l+1)}
$$

After one more epoch, all the activations $h_{CV,i,v}^{(l+1)}$ are computed at least once for each $v$, so $\bar{H}_{CV,i}^{(l+1)} = H_{CV,i}^{(l+1)} = H^{(l+1)}$ for all $i > (l+2)I$. By induction, we know that after $LI$ steps, we have $\bar{H}_{CV,i}^{(L-1)} = H_{CV,i}^{(L-1)} = H^{(L-1)}$. By Eq. 1 we also have $\bar{Z}_{CV,i}^{(L)} = Z^{(L)}$.

□

# C Proof of Theorem 2

We proof Theorem 2 in 3 steps:

1. Lemma 1: For a sequence of weights $W^{(1)}, \dots, W^{(N)}$ which are close to each other, CV's approximate activations are close to the exact activations.
2. Lemma 2: For a sequence of weights $W^{(1)}, \dots, W^{(N)}$ which are close to each other, CV's gradients are close to be unbiased.
3. Theorem 2: An SGD algorithm generates the weights that changes slow enough for the gradient bias goes to zero, so the algorithm converges.

The following proposition is needed in our proof

**Proposition B.** *Let* $\|A\|_\infty = \max_{ij} |A_{ij}|$*, then*

- $\|AB\|_\infty \le col(A) \|A\|_\infty \|B\|_\infty$*, where* $col(A)$ *is the number of columns of the matrix* $A$*.*
- $\|A \circ B\|_\infty \le \|A\|_\infty \|B\|_\infty$*, where* $\circ$ *is the element wise product.*
- $\|A + B\|_\infty \le \|A\|_\infty + \|B\|_\infty$*.*

*Proof.*

$$\|AB\|_\infty = \max_{ij} \left| \sum_k A_{ik} B_{ik} \right| \le \max_{ij} \left| \sum_k \|A\|_\infty \|B\|_\infty \right| = col(A) \|A\|_\infty \|B\|_\infty .$$

$$\|A \circ B\|_\infty = \max_{ij} |A_{ij} B_{ij}| \le \max_{ij} \|A\|_\infty \|B\|_\infty = \|A\|_\infty \|B\|_\infty .$$

$$\|A + B\|_\infty = \max_{ij} |A_{ij} + B_{ij}| \le \max_{ij} \{|A_{ij}| + |B_{ij}|\} \le \max_{ij} |A_{ij}| + \max_{ij} |B_{ij}| = \|A\|_\infty + \|B\|_\infty .$$

□

We define $C := \max\{col(P), col(H^{(0)}), \dots, col(H^{(L)})\}$ to be the maximum number of columns we can possibly encounter in the proof.

## C.1 Single layer GCN

The following proposition states that if the inputs and the weights of an one-layer GCN with CV estimator does not change too much, then its output does not change too much, and is close to the output of an exact one-layer GCN.

**Proposition C.** *If the activation* $\sigma(\cdot)$ *is* $\rho$*-Lipschitz, for any series of* $T$ *inputs, weights, and stochastic propagation matrices* $(X_i, X_{CV,i}, W_i, \hat{P}_i)_{i=1}^T$*, s.t.,*

1. *all the matrices are bound by* $B$*, i.e.,* $\|X_{CV,i}\|_\infty \le B$*,* $\|X_i\|_\infty \le B$*,* $\|W_i\|_\infty \le B$ *and* $\left\|\hat{P}_i\right\|_\infty \le B$*,*

2. *the differences are bound by $\epsilon$, i.e., $\|X_{CV,i} - X_{CV,j}\|_\infty < \epsilon$, $\|X_{CV,i} - X_i\|_\infty < \epsilon$ and $\|W_i - W_j\|_\infty < \epsilon$,*

*let $P = \mathbb{E}\hat{P}_i$. If at time $i$ we feed $(X_{CV,i}, W_i, \hat{P}_i)$ to an one-layer GCN with CV estimator to evaluate the prediction for nodes in the minibatch $\mathcal{V}_i$,* [1]

$$Z_{CV,i} = \left(\hat{P}_i(X_{CV,i} - \bar{X}_{CV,i}) + P\bar{X}_{CV,i}\right) W_i, \quad H_{CV,i} = \sigma(Z_{CV,i}).$$

*where $\bar{X}_{CV,i}$ is the maintained history at time $i$, and $(X_i, W_i, P)$ to an one-layer GCN with exact estimator*

$$Z_i = PX_iW_i, \quad H_i = \sigma(Z_i),$$

*then there exists $K$ that depends on $C$, $B$ and $\rho$, s.t. for all $I < i, j \le T$, where $I$ is the number of iterations per epoch:*

1. *The outputs does not change too fast: $\|Z_{CV,i} - Z_{CV,j}\|_\infty < K\epsilon$ and $\|H_{CV,i} - H_{CV,j}\|_\infty < K\epsilon$,*

2. *The outputs are close to the exact output: $\|Z_{CV,i} - Z_i\|_\infty < K\epsilon$ and $\|H_{CV,i} - H_i\|_\infty < K\epsilon$.*

*Proof.* Because for all $i > I$ (i.e., after one epoch), the elements of $\bar{X}_{CV,i}$ are all taken from previous iterations, i.e., $X_{CV,1}, \dots, X_{CV,i-1}$, we know that

$$\left\|\bar{X}_{CV,i} - X_{CV,i}\right\|_\infty \le \max_{j \le i} \|X_{CV,j} - X_{CV,i}\|_\infty \le \epsilon \quad (\forall i > I). \tag{2}$$

By triangular inequality, we also know

$$\left\|\bar{X}_{CV,i} - \bar{X}_{CV,j}\right\|_\infty < 3\epsilon \quad (\forall i, j > I). \tag{3}$$

$$\left\|\bar{X}_{CV,i} - X_i\right\|_\infty < 2\epsilon \quad (\forall i > I). \tag{4}$$

Since $\|X_{CV,1}\|_\infty, \dots, \|X_{CV,T}\|_\infty$ are bounded by $B$, $\left\|\bar{X}_{CV,i}\right\|_\infty$ is also bounded

[1] Conceptually we feed the data for all the nodes in $\mathcal{V}$, but since we only require the predictions for the nodes in $\mathcal{V}_i$, the algorithm will only fetch the input of a subset of nodes $\subset \mathcal{V}$, and update history for those nodes.

by $B$ for $i > I$. Then,

$$
\begin{aligned}
&\|Z_{CV,i} - Z_{CV,j}\|_\infty \\
=&\left\|\left(\hat{P}_i(X_{CV,i} - \bar{X}_{CV,i}) + P\bar{X}_{CV,i}\right)W_i - \left(\hat{P}_j(X_{CV,j} - \bar{X}_{CV,j}) + P\bar{X}_{CV,j}\right)W_j\right\|_\infty \\
\le&\left\|\hat{P}_i(X_{CV,i} - \bar{X}_{CV,i})W_i - \hat{P}_j(X_{CV,j} - \bar{X}_{CV,j})W_j\right\|_\infty + \rho\left\|P\bar{X}_{CV,i}W_i - P\bar{X}_{CV,j}W_j\right\|_\infty \\
\le&C^2[\left\|\hat{P}_i - \hat{P}_j\right\|_\infty \left\|X_{CV,i} - \bar{X}_{CV,i}\right\|_\infty \|W_i\|_\infty \\
&+ \left\|\hat{P}_j\right\|_\infty \left\|X_{CV,i} - \bar{X}_{CV,i} - X_{CV,j} + \bar{X}_{CV,j}\right\|_\infty \|W_i\|_\infty \\
&+ \left\|\hat{P}_j\right\|_\infty \left\|X_{CV,j} - \bar{X}_{CV,j}\right\|_\infty \|W_i - W_j\|_\infty \\
&+ \|P\|_\infty \left\|\bar{X}_{CV,i} - \bar{X}_{CV,j}\right\|_\infty \|W_i\|_\infty \\
&+ \|P\|_\infty \left\|\bar{X}_{CV,j}\right\|_\infty \|W_i - W_j\|_\infty] \\
\le&C^2\epsilon[\left\|\hat{P}_i - \hat{P}_j\right\|_\infty \|W_i\|_\infty + 2\left\|\hat{P}_j\right\|_\infty \|W_i\|_\infty + \left\|\hat{P}_j\right\|_\infty \|W_i - W_j\|_\infty \\
&+3\left\|\hat{P}_j\right\|_\infty \|W_i\|_\infty + \left\|\hat{P}_j\right\|_\infty \left\|\bar{X}_{CV,j}\right\|_\infty] \\
\le&\epsilon C^2\left[2B^2 + 2B^2 + 2B^2 + 3B^2 + B^2\right] \\
=&K_1\epsilon,
\end{aligned}
$$

where $K_1 = 10C^2B^2$, and

$$
\begin{aligned}
\|Z_{CV,i} - Z_i\|_\infty &\le \left\|\left(\hat{P}_i(X_{CV,i} - \bar{X}_{CV,i}) + P(\bar{X}_{CV,i} - X_i)\right)\right\|_\infty \|W_i\|_\infty \\
&\le C(\left\|\hat{P}_i\right\|_\infty \epsilon + 2\|P\|_\infty \epsilon)\|W_i\|_\infty \\
&\le 3CB^2\epsilon \\
&= K_2\epsilon,
\end{aligned}
$$

where $K_2 = 3CB^2$. By Lipschitz continuity

$$
\begin{aligned}
\|H_{CV,i} - H_{CV,j}\|_\infty &\le \rho K_1\epsilon, \\
\|H_{CV,i} - H_i\|_\infty &\le \rho K_2\epsilon.
\end{aligned}
$$

We just let $K = \max\{\rho K_1, \rho K_2, K_1, K_2\}$. □

## C.2 Lemma 1: Activation of Multi-layer GCN

The following lemma bounds the approximation error of activations in a multi-layer GCN with CV. Intuitively, there is a sequence of slow-changing model parameters $(W_i)$, where $W_i$ is the model at the $i$-th iteration. At each iteration $i$ we use GCN with CV and GCN with Exact estimator to compute the activations for the minibatch $\mathcal{V}_i$, and update the corresponding history. Then after $L$ epochs, the error of the predictions by the CV estimator is bounded by the rate of change of $(W_i)$, regardless of the stochastic propagation matrix $\hat{P}_i$.

**Lemma 1.** *Assume all the activations are $\rho$-Lipschitz, given a fixed dataset $X$ and a sequence of $T$ model weights and stochastic propagation matrices $(W_i, \hat{P}_i)_{i=1}^T$, s.t.,*

1. $\|W_i\|_\infty \leq B$ *and* $\left\|\hat{P}_i\right\|_\infty \leq B$,
2. $\|W_i - W_j\|_\infty < \epsilon, \forall i, j$,

*let $P = \mathbb{E}\hat{P}_i$. If at time $i$ we feed $(X, W_i, \hat{P}_i)$ to a GCN with CV estimator to evaluate the prediction for nodes in the minibatch $\mathcal{V}_i$,*

$$Z_{CV,i}^{(l+1)} = \left(\hat{P}_i^{(l)}(H_{CV,i}^{(l)} - \bar{H}_{CV,i}^{(l)}) + P\bar{H}_{CV,i}^{(l)}\right) W_i^{(l)}, \quad H_{CV,i}^{(l+1)} = \sigma(Z_{CV,i}^{(l+1)}).$$

*where $\bar{H}_{CV,i}^{(l)}$ is the maintained history at time $i$, and $(X, W_i, P)$ to a GCN with exact estimator*

$$Z_i^{(l+1)} = PH_i^{(l)}W_i^{(l)}, \quad H_i^{(l+1)} = \sigma(Z_i^{(l+1)}),$$

*then there exists $K$ that depends on $C$, $B$ and $\rho$ s.t.,*

- $\left\|H_i^{(L)} - H_{CV,i}^{(L)}\right\|_\infty < K\epsilon, \forall i > LI, l = 1, \ldots, L-1,$
- $\left\|Z_i^{(L)} - Z_{CV,i}^{(L)}\right\|_\infty < K\epsilon, \forall i > LI, l = 1, \ldots, L.$

*Proof.* By Proposition C.1, we know there exists $K^{(1)}$, s.t., $\left\|H_i^{(1)} - H_{CV,i}^{(1)}\right\| < K^{(1)}\epsilon$ and $\left\|H_{CV,i}^{(1)} - H_{CV,j}^{(1)}\right\| < K^{(1)}\epsilon$, $\forall i > I$.

Repeat this for $L-1$ times, we know there exist $K^{(1)}, \ldots, K^{(L)}$, s.t., $\left\|H_i^{(L)} - H_{CV,i}^{(L)}\right\| < K\epsilon$, $\left\|H_{CV,i}^{(L)} - H_{CV,j}^{(K)}\right\| < K\epsilon$, $\left\|Z_i^{(L)} - Z_{CV,i}^{(L)}\right\| < K\epsilon$ and $\left\|Z_{CV,i}^{(L)} - Z_{CV,j}^{(K)}\right\| < K\epsilon$, $\forall i > LI$, where $K = \prod_{l=1}^L K^{(l)}$.

□

## C.3 Lemma 2: Gradient of Multi-layer GCN

We reiterate some notations defined in Sec. 4 of the main text. $\mathcal{V}_i$ is the minibatch of nodes at iteration $i$ that we would like to evaluate the predictions and gradients on. $g_{CV,v}(W_i) := \nabla f(y_v, z_{CV,i,v}^{(L)})$ is the stochastic gradient propagated through the node $v$ by the CV estimator, and $g_{CV,i}(W_i) := \frac{1}{|\mathcal{V}_i|}\sum_{v\in\mathcal{V}_i} \nabla f(y_v, z_{CV,i,v}^{(L)})$ is the minibatch gradient by CV. $g_v(W_i) := \nabla f(y_v, z_v^{(L)})$ is stochastic gradient propagated through the node $v$ by the Exact estimator, and $g_i(W_i) := \frac{1}{|\mathcal{V}_i|}\sum_{v\in\mathcal{V}_i} \nabla f(y_v, z_v^{(L)})$ is the minibatch gradient by the Exact estimator. Finally, $\nabla\mathcal{L}(W_i) = \frac{1}{|\mathcal{V}_\mathcal{L}|}\sum_{v\in\mathcal{V}_\mathcal{L}} \nabla f(y_v, z_{i,v}^{(L)})$ is the exact full-batch gradient.

The following lemma bounds the bias of the gradients by the CV estimator. Intuitively, there is a sequence of slow-changing model parameters $(W_i)$, where

$W_i$ is the model at the $i$-th iteration. At each iteration $i$ we use GCN with CV and GCN with Exact estimator to compute the activations for the minibatch $\mathcal{V}_i$, and update the corresponding history. After $L$ epochs, we compute the gradient by backpropagating through CV's predictions on the minibatch of nodes $\mathcal{V}_i$. The gradient $g_{CV,i}(W_i)$ is a random variable of both the stochastic propagation matrix $\hat{P}_i$ and the minibatch $\mathcal{V}_i$. But the expectation of the gradient w.r.t. $\hat{P}_i$ and $\mathcal{V}_i$, $\mathbb{E}_{\hat{P}_i,\mathcal{V}_i} g_{CV,i}(W_i)$, is close to the full-batch gradient by the Exact estimator $\nabla\mathcal{L}(W_i)$, i.e., the gradient is close to be unbiased.

To study the gradient, we need the backpropagation rules of the networks. Let $f_v = f(y_v, z_v^{(L)})$ and $f_{CV,i,v} = f(y_z, z_{CV,i,v}^{(L)})$, we first derive the backpropagation rule for the exact algorithm. Differentiating both sides of Eq. (1), we have:

$$\begin{aligned}
\nabla_{H^{(l)}} f_v &= P^\top \nabla_{Z^{(l+1)}} f_v W^{(l)\top} && l = 1, \ldots, L-1 \\
\nabla_{Z^{(l)}} f_v &= \sigma'(Z^{(l)}) \circ \nabla_{H^{(l)}} f_v && l = 1, \ldots, L-1 \\
\nabla_{W^{(l)}} f_v &= (PH^{(l)})^\top \nabla_{Z^{(l+1)}} f_v && l = 0, \ldots, L-1.
\end{aligned} \tag{5}$$

Similarly, differentiating both sides of Eq. (5), we have

$$\begin{aligned}
\nabla_{H_{CV}^{(l)}} f_{CV,v} &= \hat{P}^{(l)} \nabla_{Z_{CV}^{(l+1)}} f_{CV,v} W^{(l)\top} && l = 1, \ldots, L-1 \\
\nabla_{Z_{CV}^{(l)}} f_{CV,v} &= \sigma'(Z_{CV}^{(l)}) \circ \nabla_{H_{CV}^{(l)}} f_{CV,v} && l = 1, \ldots, L-1 \\
\nabla_{W^{(l)}} f_{CV,v} &= (\hat{P}^{(l)} H_{CV}^{(l)})^\top \nabla_{Z_{CV}^{(l+1)}} f_{CV,v} && l = 0, \ldots, L-1.
\end{aligned} \tag{6}$$

**Lemma 2.** *Assume $\sigma(\cdot)$ and $\nabla_z f(y,z)$ are $\rho$-Lipschitz, $\|\nabla_z f(y,z)\|_\infty \le B$. Given a fixed dataset $X$ and a sequence of $T$ weights and stochastic propagation matrices $(W_i, \hat{P}_i)_{i=1}^T$, s.t.,*

1. *$\|W_i\|_\infty \le B$, $\left\|\hat{P}_i\right\|_\infty \le B$, and $\|\sigma'(Z_{CV,i})\|_\infty \le B$,*
2. *$\|W_i - W_j\|_\infty < \epsilon, \forall i, j$,*

*let $P = \mathbb{E}\hat{P}_i$. If at time $i$ we feed $(X, W_i, \hat{P}_i)$ to a GCN with CV estimator to evaluate the prediction for nodes in the minibatch $\mathcal{V}_i$,*

$$Z_{CV,i}^{(l+1)} = \left(\hat{P}_i^{(l)}(H_{CV,i}^{(l)} - \bar{H}_{CV,i}^{(l)}) + P\bar{H}_{CV,i}^{(l)}\right) W_i^{(l)}, \quad H_{CV,i}^{(l+1)} = \sigma(Z_{CV,i}^{(l+1)}).$$

*where $\bar{H}_{CV,i}^{(l)}$ is the maintained history at time $i$, and $(X, W_i, P)$ to a GCN with exact estimator*

$$Z_i^{(l+1)} = PH_i^{(l)} W_i^{(l)}, \quad H_i^{(l+1)} = \sigma(Z_i^{(l+1)}),$$

*then there exists $K$ that depends on $C$, $B$ and $\rho$ s.t.,*

$$\left\|\mathbb{E}_{\hat{P}_i,\mathcal{V}_i}(W_i) - \nabla\mathcal{L}(W_i)\right\|_\infty \le K\epsilon, \forall i > LI.$$

*Proof.* By Lipschitz continuity of $\nabla_z f(y,z)$ and Lemma 1, there exists $\dot{K}$, for all $\hat{P}_i = (\hat{P}_i^{(0)}, \dots, \hat{P}_i^{(L-1)})$

$$\begin{aligned}
&\left\|\nabla_{z_{CV,v}^{(L)}} f_{CV,v} - \nabla_{z_v^{(L)}} f_v\right\|_\infty \\
\le&\rho \left\|z_{CV,v}^{(L)} - z_v^{(L)}\right\|_\infty \\
\le&\rho \dot{K} \epsilon, \\
\left\|\sigma'(Z_{CV}^{(l)}) - \sigma'(Z^{(l)})\right\|_\infty \le&\rho \dot{K} \epsilon
\end{aligned} \tag{7}$$

We prove by induction that there exists $K_l$, s.t., $\forall l \in [L]$,,

$$\left\|\mathbb{E}_{\hat{P}^{(\ge l)}} \nabla z_{CV,v}^{(l)} f_{CV,v} - \nabla z_v^{(l)} f_v\right\|_\infty \le K_l \epsilon, \quad \forall \hat{P}^{(0)}, \dots, \hat{P}^{(l-1)}, \tag{8}$$

where $\hat{P}^{(\ge l)} = (\hat{P}^{(l)}, \dots, \hat{P}^{(L-1)})$. By Eq. (7) the statement holds for $l = L$, where $K_L = \rho \dot{K}$. If the statement holds for $l+1$, i.e.,

$$\left\|\mathbb{E}_{\hat{P}^{(\ge l+1)}} \nabla z_{CV,v}^{(l+1)} f_{CV,v} - \nabla z_v^{(l+1)} f_v\right\|_\infty \le K_l \epsilon, \quad \forall \hat{P}^{(0)}, \dots, \hat{P}^{(l)},$$

then by Eq. (5, 6),

$$\begin{aligned}
&\left\|\mathbb{E}_{\hat{P}^{(\ge l)}} \nabla z_{CV,v}^{(l)} f_{CV,v} - \nabla z_v^{(l)} f_v\right\|_\infty \\
=&\left\|\mathbb{E}_{\hat{P}^{(\ge l)}} \sigma'(Z_{CV}^{(l)}) \circ \hat{P}^{(l)} \nabla_{Z_{CV}^{(l+1)}} f_{CV,v} - \sigma'(Z^{(l)}) \circ P^\top \nabla_{Z^{(l+1)}} f_v\right\|_\infty \\
=&\left\|\mathbb{E}_{\hat{P}^{(\ge l)}} \left\{\left[\sigma'(Z_{CV}^{(l)}) \circ \hat{P}^{(l)} \nabla_{Z_{CV}^{(l+1)}} f_{CV,v}\right] - \sigma'(Z^{(l)}) \circ P^\top \nabla_{Z^{(l+1)}} f_v\right\}\right\|_\infty \\
\le&\left\|\mathbb{E}_{\hat{P}^{(\ge l)}} \left\{\left[\left(\sigma'(Z_{CV}^{(l)}) - \sigma'(Z^{(l)})\right) \circ \hat{P}^{(l)} \nabla_{Z_{CV}^{(l+1)}} f_{CV,v}\right]\right\}\right\|_\infty \\
&+ \mathbb{E}_{\hat{P}^{(l)}} \left\|\mathbb{E}_{\hat{P}^{(\ge l+1)}} \left[\sigma'(Z^{(l)}) \circ \hat{P}^{(l)} \left(\nabla_{Z_{CV}^{(l+1)}} f_{CV,v} - \nabla_{Z^{(l+1)}} f_v\right)\right]\right\|_\infty \\
&+ \left\|\mathbb{E}_{\hat{P}^{(\ge l)}} \left\{\left[\sigma'(Z^{(l)}) \circ \left(\hat{P}^{(l)} - P^\top\right) \nabla_{Z^{(l+1)}} f_v\right]\right\}\right\|_\infty \\
\le&\mathbb{E}_{\hat{P}^{(\ge l)}} \left[\left\|\sigma'(Z_{CV}^{(l)}) - \sigma'(Z^{(l)})\right\|_\infty \left\|\hat{P}^{(l)} \nabla_{Z_{CV}^{(l+1)}} f_{CV,v}\right\|_\infty\right] \\
&+ \mathbb{E}_{\hat{P}^{(l)}} \left\|\sigma'(Z^{(l)})\right\|_\infty \mathbb{E}_{\hat{P}^{(\ge l+1)}} \left\|\hat{P}^{(l)}\right\|_\infty \mathbb{E}_{\hat{P}^{(\ge l+1)}} \left\|\nabla_{Z_{CV}^{(l+1)}} f_{CV,v} - \nabla_{Z^{(l+1)}} f_v\right\|_\infty \\
&+ 0 \\
\le&\rho \dot{K} \epsilon B^2 C^2 + B^2 C^2 K_{l+1} \epsilon \\
=&K_l \epsilon,
\end{aligned}$$

where $K_l = B^2 C^2 (\rho \dot{K} + K_{l+1})$. By induction, Eq. (8) holds. Similarly, we can show that there exists $K$, s.t.,

$$\left\|\mathbb{E}_{\hat{P}} \nabla_{W^{(l)}} f_{CV,v} - \nabla_{W^{(l)}} f_v\right\|_\infty < K \epsilon, \quad \forall l \in [L-1].$$

Therefore,

$$
\begin{aligned}
&\left\|\mathbb{E}_{\mathcal{V}_i,\hat{P}_i} g_{CV,i}(W_i) - \nabla\mathcal{L}(W_i)\right\|_\infty \\
=&\left\|\mathbb{E}_{v\in\mathcal{V},\hat{P}_i} g_{CV,v}(W_i) - \mathbb{E}_{v\in\mathcal{V}} g_v(W_i)\right\|_\infty \\
\le&\mathbb{E}_{\mathcal{V}_i}\left\|\mathbb{E}_{\hat{P}_i} g_{CV,v}(W_i) - g_v(W_i)\right\|_\infty \\
\le&\mathbb{E}_{\mathcal{V}_i}\max_l \left\|\mathbb{E}_{\hat{P}}\nabla_{W^{(l)}} f_{CV,v} - \nabla_{W^{(l)}} f_v\right\|_\infty \\
\le&K\epsilon.
\end{aligned}
$$

□

### C.4 Proof of Theorem 2

**Theorem 2.** *Assume that (1) the activation $\sigma(\cdot)$ is $\rho$-Lipschitz, (2) the gradient of the cost function $\nabla_z f(y,z)$ is $\rho$-Lipschitz and bounded, (3) $\|g_{CV,\mathcal{V}}(W)\|_\infty$, $\|g(W)\|_\infty$, and $\|\nabla\mathcal{L}(W)\|_\infty$ are all bounded by $G>0$ for all $\hat{P},\mathcal{V}$ and $W$. (4) The loss $\mathcal{L}(W)$ is $\rho$-smooth, i.e., $|\mathcal{L}(W_2)-\mathcal{L}(W_1)-\langle\nabla\mathcal{L}(W_1),W_2-W_1\rangle| \le \frac{\rho}{2}\|W_2-W_1\|_F^2\ \forall W_1,W_2$, where $\langle A,B\rangle = tr(A^\top B)$ is the inner product of matrix $A$ and matrix $B$. Then, there exists $K>0$, s.t., $\forall N > LI$, if we run SGD for $R\le N$ iterations, where $R$ is chosen uniformly from $[N]_+$, we have*

$$
\mathbb{E}_R\|\nabla\mathcal{L}(W_R)\|_F^2 \le 2\frac{\mathcal{L}(W_1)-\mathcal{L}(W^*)+K+\rho K}{\sqrt{N}},
$$

*for the updates $W_{i+1}=W_i-\gamma g_{CV,i}(W_i)$ and the step size $\gamma=\min\{\frac{1}{\rho},\frac{1}{\sqrt{N}}\}$.*

*Proof.* This proof is a modification of [2], but using biased stochastic gradients instead. We assume the algorithm is already warmed-up for $LI$ steps with the initial weights $W_0$, so that Lemma 2 holds for step $i>0$. Denote $\delta_i = g_{CV,i}(W_i)-\nabla\mathcal{L}(W_i)$. By smoothness we have

$$
\begin{aligned}
\mathcal{L}(W_{i+1}) &\le \mathcal{L}(W_i) + \langle\nabla\mathcal{L}(W_i), W_{i+1}-W_i\rangle + \frac{\rho}{2}\gamma^2\|g_{CV,i}(W_i)\|_F^2 \\
&= \mathcal{L}(W_i) - \gamma\langle\nabla\mathcal{L}(W_i), g_{CV,i}(W_i)\rangle + \frac{\rho}{2}\gamma^2\|g_{CV,i}(W_i)\|_F^2 \\
&= \mathcal{L}(W_i) - \gamma\langle\nabla\mathcal{L}(W_i),\delta_i\rangle - \gamma\|\nabla\mathcal{L}(W_i)\|^2 + \frac{\rho}{2}\gamma^2\left[\|\delta_i\|^2 + \|\nabla\mathcal{L}(W_i)\|_F^2 + 2\langle\delta_i,\nabla\mathcal{L}(W_i)\rangle\right] \\
&= \mathcal{L}(W_i) - (\gamma-\rho\gamma^2)\langle\nabla\mathcal{L}(W_i),\delta_i\rangle - (\gamma-\frac{\rho\gamma^2}{2})\|\nabla\mathcal{L}(W_i)\|_F^2 + \frac{\rho}{2}\gamma^2\|\delta_i\|_F^2.
\end{aligned}
\tag{9}
$$

For each $i$, consider the sequence of $LI+1$ weights $W_{i-LI}, \ldots, W_i$.

$$\max_{i-LI\le j,k\le i} \|W_j - W_k\|_\infty \le \sum_{j=i-LI}^{i-1} \|W_j - W_{j+1}\|_\infty$$
$$= \sum_{j=i-LI}^{i-1} \gamma \|g_{CV}(W_j)\|_\infty \le \sum_{j=i-LI}^{i-1} \gamma G = LIG\gamma.$$

By Lemma 2, there exists $\dot{K} > 0$, s.t.

$$\left\|\mathbb{E}_{\hat{P},\mathcal{V}_B}\delta_i\right\|_\infty = \left\|\mathbb{E}_{\hat{P},\mathcal{V}_B} g_{CV}(W_i) - \nabla\mathcal{L}(W_i)\right\|_\infty \le \dot{K}LIG\gamma, \quad \forall i > 0.$$

Assume that $W$ is $D$-dimensional,

$$\mathbb{E}_{\hat{P},\mathcal{V}_B}\langle\nabla\mathcal{L}(W_i), \delta_i\rangle \le D\|\nabla\mathcal{L}(W_i)\|_\infty \left\|\mathbb{E}_{\hat{P},\mathcal{V}_B}\delta_i\right\|_\infty \le \dot{K}LIDG^2\gamma \le K\gamma,$$
$$\mathbb{E}_{\hat{P},\mathcal{V}_B}\|\delta_i\|_F^2 \le D\|g_{CV,i}(W_i)\|_\infty + D\|\nabla\mathcal{L}(W_i)\|_\infty \le 2DG^2 \le K,$$

where $K = \max\{\dot{K}LIDG^2, 2DG^2\}$. Taking $\mathbb{E}_{\hat{P},\mathcal{V}_B}$ to both sides of Eq. 9 we have

$$\mathcal{L}(W_{i+1}) \le \mathcal{L}(W_i) + (\gamma - \rho\gamma^2)K\gamma - (\gamma - \frac{\rho\gamma^2}{2})\|\nabla\mathcal{L}(W_i)\|_F^2 + \rho K\gamma^2/2.$$

Summing up the above inequalities and re-arranging the terms, we obtain,

$$(\gamma - \frac{\rho\gamma^2}{2})\sum_i \|\nabla\mathcal{L}(W_i)\|_F^2$$
$$\le \mathcal{L}(W_1) - \mathcal{L}(W^*) + KN(\gamma - \rho\gamma^2)\gamma + \frac{\rho K}{2}N\gamma^2.$$

Dividing both sides by $N(\gamma - \frac{\rho\gamma^2}{2})$, and take $\gamma = \min\{\frac{1}{\rho}, \frac{1}{\sqrt{N}}\}$

$$\mathbb{E}_{R\sim P_R}\|\nabla\mathcal{L}(W_R)\|_F^2$$
$$\le 2\frac{\mathcal{L}(W_1) - \mathcal{L}(W^*) + KN(\gamma - \rho\gamma^2)\gamma + \frac{\rho K}{2}N\gamma^2}{N\gamma(2-\rho\gamma)}$$
$$\le 2\frac{\mathcal{L}(W_1) - \mathcal{L}(W^*) + KN(\gamma - \rho\gamma^2)\gamma + \frac{\rho K}{2}N\gamma^2}{N\gamma}$$
$$\le 2\frac{\mathcal{L}(W_1) - \mathcal{L}(W^*)}{N\gamma} + K\gamma(1-\rho\gamma) + \rho K\gamma$$
$$\le 2\frac{\mathcal{L}(W_1) - \mathcal{L}(W^*)}{\sqrt{N}} + K\gamma + \rho K/\sqrt{N}$$
$$\le 2\frac{\mathcal{L}(W_1) - \mathcal{L}(W^*) + K + \rho K}{\sqrt{N}}.$$

Particularly, when $N \to \infty$, we have $\mathbb{E}_{R\sim P_R}\|\nabla\mathcal{L}(W_R)\|_F^2 = 0$, which implies that the gradient is asymptotically unbiased.

□

**Algorithm 1** Constructing the receptive fields and random propagation matrices.

$\mathbf{r}^{(L)} \leftarrow \mathcal{V}_B$
**for** layer $l \leftarrow L-1$ to $0$ **do**
  $\mathbf{r}^{(l)} \leftarrow \varnothing$
  $\hat{P}^{(l)} \leftarrow \mathbf{0}$
  **for** each node $u \in \mathbf{r}^{(l+1)}$ **do**
    $\mathbf{r}^{(l)} \leftarrow \mathbf{r}^{(l)} \cup \{u\}$
    $\hat{P}^{(l)}_{uu} \leftarrow \hat{P}^{(l)}_{uu} + P_{uu} n(u)/D^{(l)}$
    **for** $D^{(l)}-1$ random neighbors $v \in \mathbf{n}(u)$ **do**
      $\mathbf{r}^{(l)} \leftarrow \mathbf{r}^{(l)} \cup \{v\}$
      $\hat{P}^{(l)}_{uv} \leftarrow \hat{P}^{(l)}_{uv} + P_{uv} n(u)/D^{(l)}$
    **end for**
  **end for**
**end for**

# D Pseudocode

As mentioned in Sec. 3.3, an iteration of our algorithm consists the following operations:

1. Randomly select a minibatch $\mathcal{V}_B \in \mathcal{V}_L$ of nodes;
2. Build a computation graph that only contains the activations $h^{(l)}_v$ and $\bar{h}^{(l)}_v$ needed for the current minibatch;
3. Get the predictions by forward propagation as Eq. (6) in the main text;
4. Get the gradients by backward propagation, and update the parameters by SGD;
5. Update the historical activations.

For step 2, we construct the receptive fields $\mathbf{r}^{(l)}$ and stochastic propagation matrices $\hat{P}^{(l)}$ as Alg. 1.

## D.1 Training with the CV estimator

Alg. 2 depicts the training algorithm using the CV estimator. We perform forward propagation according to Eq. (6), compute the stochastic gradient, and then update the historical activations $\bar{H}^{(l)}$ for all the nodes in $\mathbf{r}^{(l)}$. Let $W = (W^{(0)}, \ldots, W^{(L-1)})$ be all the trainable parameters, the gradient $\nabla_W \mathcal{L}$ is computed automatically by frameworks such as TensorFlow.

**Algorithm 2** Training with the CV algorithm

**for** each minibatch $\mathcal{V}_B \subset \mathcal{V}$ **do**
  Compute the receptive fields $\mathbf{r}^{(l)}$ and stochastic propagation matrices $\hat{P}^{(l)}$ as Alg. 1.
  (Forward propgation)
  **for** each layer $l \leftarrow 0$ to $L-1$ **do**
    $Z^{(l+1)} \leftarrow \left(\hat{P}^{(l)}(H^{(l)} - \bar{H}^{(l)} + P\bar{H}^{(l)}\right) W^{(l)}$
    $H^{(l+1)} \leftarrow \sigma(Z^{(l+1)})$
  **end for**
  Compute the loss $\mathcal{L} = \frac{1}{|\mathcal{V}_B|}\sum_{v\in\mathcal{V}_B} f(y_v, Z_v^{(L)})$
  (Backward propagation)
  $W \leftarrow W - \gamma_i \nabla_W \mathcal{L}$
  (Update historical activations)
  **for** each layer $l \leftarrow 0$ to $L-1$ **do**
    **for** each node $v \in \mathbf{r}^{(l)}$ **do**
      $\bar{h}_v^{(l)} \leftarrow h_v^{(l)}$
    **end for**
  **end for**
**end for**

### D.2 Training with the CVD estimator

Training with the CVD estimator is similar with the CV estimator, except it runs two versions of the network, with and without dropout, to compute the samples $H$ and their mean $\mu$ of the activation. The matrix $\bar{P}_{uv}^{(l)} = \hat{P}_{uv}^{(l)}/\sqrt{n(v)}$ , where $n(v)$ is the degree of node $v$.

## E Experiment setup

In this sections we describe the details of our model architectures. We use the Adam optimizer [4] with learning rate 0.01.

- Citeseer, Cora, PubMed and NELL: We use the same architecture as [5]: two graph convolution layers with one linear layer per graph convolution layer. We use 32 hidden units, 50% dropout rate and $5 \times 10^{-4}$ L2 weight decay for Citeseer, Cora and PubMed and 64 hidden units, 10% dropout rate and $10^{-5}$ L2 weight decay for NELL.

- PPI and Reddit: We use the mean pooling architecture GraphSAGE-mean proposed by [3]. We use two linear layers per graph convolution layer. We set weight decay as zero, dropout rate as 20%, and adopt layer normalization [1] after each linear layer. We use 512 hidden units for PPI and 128 hidden units for Reddit. We find that our architecture can reach 97.8% testing micro-F1 on the PPI dataset, which is significantly higher

**Algorithm 3** Training with the CVD algorithm

**for** each minibatch $\mathcal{V}_B \subset \mathcal{V}$ **do**
  Compute the receptive fields $\mathbf{r}^{(l)}$ and stochastic propagation matrices $\hat{P}^{(l)}$ as Alg. 1.
  (Forward propgation)
  **for** each layer $l \leftarrow 0$ to $L-1$ **do**
    $U \leftarrow \left(\bar{P}^{(l)}(H^{(l)} - \mu^{(l)}) + \hat{P}^{(l)}(\mu^{(l)} - \bar{\mu}^{(l)}) + P\bar{H}^{(l)}\right)$
    $H^{(l+1)} \leftarrow \sigma(\mathrm{Dropout}_p(U)W^{(l)})$
    $\mu^{(l+1)} \leftarrow \sigma(UW^{(l)})$
  **end for**
  Compute the loss $\mathcal{L} = \frac{1}{|\mathcal{V}_B|}\sum_{v\in\mathcal{V}_B} f(y_v, H_v^{(L)})$
  (Backward propagation)
  $W \leftarrow W - \gamma_i \nabla_W \mathcal{L}$
  (Update historical activations)
  **for** each layer $l \leftarrow 0$ to $L-1$ **do**
    **for** each node $v \in \mathbf{r}^{(l)}$ **do**
      $\bar{h}_v^{(l)} \leftarrow h_v^{(l)}$
    **end for**
  **end for**
**end for**

Table 1: Time to reach 0.95 testing accuracy.

| Alg. | Valid. acc. | Epochs | Time (s) | Sparse GFLOP | Dense TFLOP |
|---|---|---|---|---|---|
| Exact | 0.940 | **3.0** | 199 | 306 | 11.7 |
| NS | 0.940 | 24.0 | 148 | 33.6 | 9.79 |
| NS+PP | 0.940 | 12.0 | 68 | **2.53** | 4.89 |
| CV+PP | 0.940 | 5.0 | **32** | 8.06 | **2.04** |
| CVD+PP | 0.940 | 5.0 | 36 | 16.1 | 4.08 |

than 59.8% reported by [3]. We find the improvement is from wider hidden layer, dropout and layer normalization.

# F Experiment for 3-layer GCNs

We test 3-layer GCNs on the Reddit dataset. The settings are the same with 2-layer GCNs in Sec. 6.2. To ensure M1+PP can run in a reasonable amount of time, we subsample the graph so that the maximum degree is 10. The convergence result is shown as Fig. 1, where the conclusion is similar with the two-layer models: CVD+PP is the best-performing approximate algorithm, followed by CV+PP, and then NS+PP and NS. The time consumption to reach 0.94 testing accuracy is shown in Table 1.

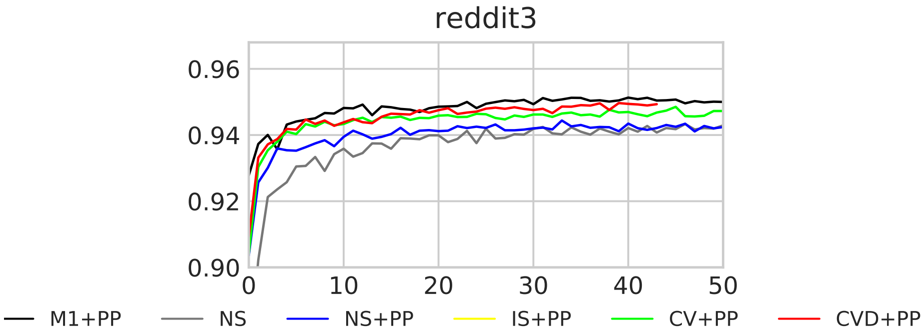


Figure 1: Comparison of validation accuracy with respect to number of epochs for 3-layer GCNs.

# G Correlation between node activations

In our analysis of the variance for the CVD estimator in Sec. 5.2, we assume that the activations for different nodes are uncorrelated, i.e., $\text{Cov}_M\left[h_u^{(l)}, h_v^{(l)}\right] = 0$, for all $u \neq v$, where $M$ is the dropout mask. We show the rationale behind this assumption in this section. For 2-layer GCNs, the activations are indeed independent, and the correlation is still weak for deeper GCNs due to the sparsity of our sampled graph.

## G.1 Results for 2-layer GCNs

For a 2-layer GCN with the first layer pre-processed, the activations of nodes are independent. Suppose we want to compute the prediction for a node on the second layer. Without loss of generality, assume that we want to compute $z_1^{(2)}$, and the neighbors of node 1 are $1, \ldots, D$. The activation $h_v^{(1)} = \sigma\left((M_v \circ u_v^{(0)})W^{(0)}\right)$, where $u_v^{(0)} = (PH^{(0)})_v$ is a random variable with respect to $M_v$, $M_v \sim \text{Bernoulli}(p)$ is the dropout mask. We show that $h_v^{(1)}$ and $h_{v'}^{(1)}$ are independent, for $v \neq v'$ by the following lemma.

**Lemma 3.** *If $a$ and $b$ are independent random variables, then their transformations $f_1(a)$ and $f_2(b)$ are independent.*

Because for any event $A$ and $B$, $P(f_1(a) \in f_1(A), f_2(b) \in f_2(B)) = P(a \in A, b \in B) = P(a \in A)P(b \in B) = P(f_1(a) \in f_1(A))P(f_2(B) \in f_2(B))$, where $f_1(A) = \{f_1(a) | a \in A\}$ and $f_2(B) = \{f_2(b) | b \in B\}$.

Let $h_v^{(1)} = f_1(M_v) := \sigma\left((M_v \circ u_v^{(0)})W^{(0)}\right)$ and $h_{v'}^{(1)} = f_1(M_{v'}) := \sigma\left((M_{v'} \circ u_{v'}^{(0)})W^{(0)}\right)$, because $M_v$ and $M_{v'}$ are independent Bernoulli random variables, $h_v^{(1)}$ and $h_{v'}^{(1)}$ are independent.

The result can be further generalized to deeper models. If the receptive fields of two nodes does not overlap, they should be independent.

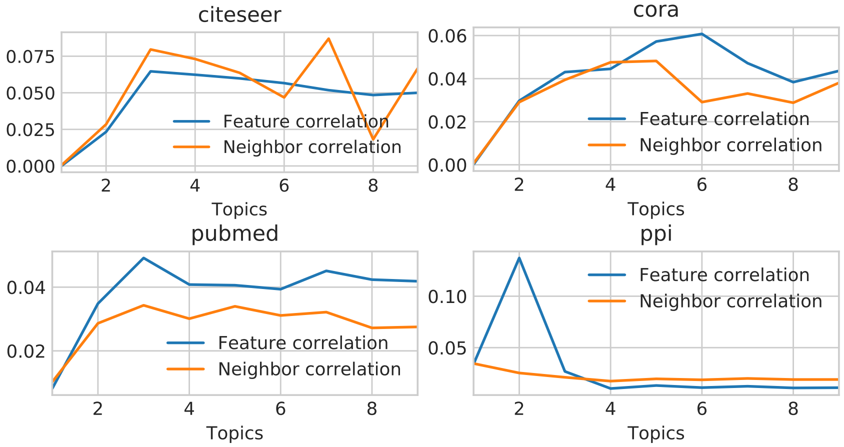

Figure 2: Average feature and neighbor correlations in a 10-layer GCN.

## G.2 Empirical results for deeper GCNs

Because we only sample two neighbors per node, the sampled subgraph is very close to a graph with all its nodes isolated, which reduces to the MLP case that [6] discuss.

We empirically study the correlation between feature dimensions and neighbors. The definition of the correlation between feature dimensions is the same with [6]. For each node $v$ on layer $l$, we compute the correlation between each feature dimension of $h_v^{(l)}$

$$\mathrm{Cov}_{ij}^{(l,v)} := \mathbb{C}[h_{vi}^{(l)}, h_{vj}^{(l)}]$$

$$\mathrm{Corr}_{ij}^{(l,v)} := \frac{\mathrm{Cov}_{ij}^{(l,v)}}{\sqrt{\mathrm{Cov}_{ii}^{(l,v)}}\sqrt{\mathrm{Cov}_{jj}^{(l,v)}}},$$

where $i$ and $j$ are the indices for different hidden dimensions, and $\mathbb{C}[X, Y] = \mathbb{E}[(X - \mathbb{E}X)(Y - \mathbb{E}Y)]$ is the covariance between two random variables $X$ and $Y$. We approximate $\mathrm{Cov}_{ij}^{(l,v)}$ with 1,000 samples of the activations $h_{vi}^{(l)}$ and $h_{vj}^{(l)}$, by running the forward propagation 1,000 times with different dropout masks. We define the *average feature correlation on layer* $l$ to be $\mathrm{Cov}_{ij}^{(l,v)}$ averaged by the nodes $v$ and dimension pairs $i \neq j$.

To compute the correlation between neighbors, we treat each feature dimension separately. For each layer $l+1$, node $v$, and dimension $d$, we compute the correlation matrix of all the activations $\{h_{id}^{(l)} | i \in \bar{\mathbf{n}}^{(l)}(v)\}$ that are needed by $h_{vd}^{(l+1)}$, where $\bar{\mathbf{n}}^{(l)}(v) = \{i | \hat{P}_{vi}^{(l)} \neq 0\}$ is the set of subsampled neighbors for node

$v$:

$$\mathrm{Cov}_{ij}^{(l,v,d)} := \mathbb{C}[h_{id}^{(l)}, h_{jd}^{(l)}]$$

$$\mathrm{Corr}_{ij}^{(l,v,d)} := \frac{\mathrm{Cov}_{ij}^{(l,v,d)}}{\sqrt{\mathrm{Cov}_{ii}^{(l,v,d)}}\sqrt{\mathrm{Cov}_{jj}^{(l,v,d)}}},$$

where the indices $i, j \in \bar{\mathbf{n}}^{(l)}(v)$. Then, we compute the average correlation of all pairs of neighbors $i \neq j$.

$$\mathrm{AvgCorr}^{(l,v,d)} := \frac{1}{\left|\bar{\mathbf{n}}^{(l)}(v)\right|\left(\left|\bar{\mathbf{n}}^{(l)}(v)\right| - 1\right)} \sum_{i \neq j} \mathrm{Corr}_{ij}^{(l,v,d)},$$

and define the *average neighbor correlation on layer* $l$ as $\mathrm{AvgCorr}^{(l,v,d)}$ averaged over all the nodes $v$ and dimensions $d$.

We report the average feature correlation and the average neighbor correlation per layer, on the Citeseer, Cora, PubMed and PPI datasets. These quantities are too expensive to compute for NELL and Reddit. On each dataset, we train a GCN with 10 graph convoluation layers until early stopping criteria is met, and compute the average feature correlation and the average neighbor correlation for layer 1 to 9. We are not interested in the correlation on layer 10 because there are no more graph convolutional layers after it. The result is shown as Fig. 2. As analyzed in Sec. G.1, the average neighbor correlation is close to zero on the first layer, but it is not exactly zero due to the finite sample size for computing the empirical covariance. There is no strong tendency of increased correlation as the number of layers increases, after the third layer. The average neighbor correlation and the average feature correlation remain on the same order of magnitude, so bringing correlated neighbors does not make the activations much more correlated than the MLP case [6]. Finally, both correlations are much smaller than one.

# References


[1] Jimmy Lei Ba, Jamie Ryan Kiros, and Geoffrey E Hinton. Layer normalization. *arXiv preprint arXiv:1607.06450*, 2016.

[2] Saeed Ghadimi and Guanghui Lan. Stochastic first-and zeroth-order methods for nonconvex stochastic programming. *SIAM Journal on Optimization*, 23(4):2341–2368, 2013.

[3] William L Hamilton, Rex Ying, and Jure Leskovec. Inductive representation learning on large graphs. *arXiv preprint arXiv:1706.02216*, 2017.

[4] Diederik Kingma and Jimmy Ba. Adam: A method for stochastic optimization. *arXiv preprint arXiv:1412.6980*, 2014.

[5] Thomas N Kipf and Max Welling. Semi-supervised classification with graph convolutional networks. In *ICLR*, 2017.

[6] Sida Wang and Christopher Manning. Fast dropout training. In *Proceedings of the 30th International Conference on Machine Learning (ICML-13)*, pages 118–126, 2013.
